# Supplementary material for: DynamicTrack: Advancing Gigapixel Tracking in Crowded Scenes
Source: arXiv:2407.18637 source file (2024-07-26)
Supplement: Supplementary file 1 [file 6_Suplement.tex]

\clearpage
\section{Supplementary Material}
\begin{figure}[t]
	\includegraphics[width=0.45\textwidth]{figures/crowd-detect.png}
	\caption{Example of dynamic detection results in different scenarios of CrowdHuman test set.}
	\label{fig:sup-crowddetect}
\end{figure}
\begin{figure}[t]
	\includegraphics[width=0.45\textwidth]{figures/panda-detect-zip.png}
	\caption{Example of dynamic detection results in different scenarios of PANDA test set.}
	\label{fig:sup-pandadetect}
\end{figure}
\subsection{Dynamic Detection}
\par \noindent \textbf{Detection Setup.}
For the detection module, we constructed a dynamic detector based on the well-known Faster-RCNN architecture. Our detector was trained using the CrowdHuman dataset, and the same training weights were utilized for subsequent experiments. 
To tackle the challenge of gigapixel detection, we employed a sliding window strategy to divide the gigapixel image into smaller portions with limited resolution. The sliding overlap was set to 0.3 to ensure comprehensive coverage. To accommodate the vast scene size, we used multiple scales, specifically $1600\times1600, 3200\times3200$ and $6400\times6400$, for the sliding window approach. The detections obtained from the different scales were fused together using Non-Maximum Suppression with a threshold of 0.7. 

\par \noindent \textbf{Sliding Window Scales.} 
The PANDA dataset covers a large range of scenes while keeping distant details clearly visible. This leads to huge variations in the size of the target in the foreground and background, posing a huge challenge for detection. To overcome this obstacle, we use different scales of sliding windows for detection and fuse candidates to obtain the final results. The results in ~\cref{tab:detection} shows the effect of different scales on the tracker. Smaller sliding windows are more effective for tracking distant background pedestrians and larger sliding windows are more accurate for tracking pedestrians in the near foreground. By combining sliding windows of different scales, the tracker can achieve robust tracking in large scenes.
\begin{figure}[t]
	\includegraphics[width=0.45\textwidth]{figures/ablation-feature_zip.png}
	\caption{Example of how head feature imporves the performance when a target is occluded.}
	\label{fig:panda-albation}
\end{figure}
\begin{table}[t]
	\centering
	\begin{tabular}{ccccc}
		\toprule
		Window scale & HOTA$\uparrow$ & MOTA$\uparrow$ & MOTP$\uparrow$ & IDF1$\uparrow$ \\
		\midrule
		3200  & 51.2 & 57.2 & 84.3 & 56.7 \\
		6400  & 36.8 & 26.2 & 86.4 & 35.9 \\
		3200+6400  & 52.0 & 57.9 & 84.4 & 57.6 \\
		\bottomrule
	\end{tabular}
	\caption{The quantitative comparison of different scales of the sliding window for gigapixel detector.}
	\label{tab:detection}
\end{table}
\par \noindent \textbf{Qualitative results.} To check the effect of matching, we chose the results in different scenarios. The boxes of the same color represent the head and body of the same pedestrian. ~\cref{fig:sup-crowddetect} shows the results of the dynamic detector on crowdhuman and ~\cref{fig:sup-pandadetect} shows the results of the dynamic detector on PANDA. The results demonstrate the robust performance of the algorithm, both under normal conditions and in densely occluded crowds.

\subsection{Dynamic Association}
\par \noindent \textbf{Performance in Crowded Scenes.}
DynamicTrack achieves robust tracking in crowded scenes by introducing head information to assist pedestrian tracking. We quantitatively demonstrate the tracker's results in ~\cref{tab:mot20-baseline} and ~\cref{tab:panda-baseline}, showing improved performance on both MOT20 and PANDA datasets. Additionally, we provide qualitative results as shown in ~\cref{fig:panda-albation}. In crowded scenes, despite severe occlusion of the target's body, its head information remains robust. By utilizing its head for assistance, our DynamicTrack enables accurate tracking of the target.

\par \noindent \textbf{Qualitative results.} More qualitative results of the PANDA dataset are shown in Fig. \ref{fig:sup-results} under different scenes. In Train Station Square and Xili Crossroad scenes, we show the tracking results in a large scene from large foreground to small background. In Xili Crossroad and University Canteen scenes, we demonstrate the robust tracking under severe occlusions and long term sequence. In Huaqiangbei scene, we demonstrate the potential of DynamicTrack with extremely dense crowds.
\begin{figure*}[t]
	\includegraphics[width=0.95\textwidth]{figures/sup-result.jpg}
	\caption{More qualitative results of DynamicTrack. We selected representative scenarios that are extremely challenging. Our DynamicTrack generates reliable tracking in large-scale long-term gigapixel sequences.}
	\label{fig:sup-results}
\end{figure*}
